# Supplementary material for: Learning Functionally Decomposed Hierarchies for Continuous Control Tasks with Path Planning
Source: arXiv:2002.05954 source file (2021-10-06)
Supplement: Supplementary file 1 [file 07_appendix.tex]

\clearpage
\label{Appendix}
\section{Environment Details}
\label{appendix_env_details}
We build on the Mujoco~\cite{todorov2012mujoco} environments used in \cite{nachum2018data}. The rewards in all experiments are sparse, i.e., $0$ for reaching the goal and ${-1}$ otherwise. We consider the goal reached if $|s-g|_{\max} < 1$. All environments use $dt=0.02$. Each episode in the simple maze navigation experiment (Section \ref{sec5_exp1}) is terminated after 500 steps and after 800 steps for the complex maze experiment (Section \ref{subsec_mazenav_complex}). In the robot manipulation experiment (Section \ref{subsec_transfer_policies}), we terminate after 800 steps and in the reacher experiments (Section \ref{sec:ext_epx}) after 200 steps. 

\subsection{Agents}
\label{subsec{agents}}
Our ant agent is equivalent to the one in \cite{levy2018hierarchical}. In other words, the ant from Rllab~\cite{duan2016benchmarking} with gear power of 16 instead of 150 and 10 frame skip instead of 5. Our ball agent is the PointMass agent from DM Control Suite~\cite{deepmindcontrolsuite2018}. We changed the joints so that the ball rolls instead of sliding. Furthermore, we resize the motor gear and the ball itself to match the maze size. For the manipulation robot, we slightly adapt the "Push" task from OpenAI gym \cite{openai_gym}. The original environment uses an inverse kinematic controller to steer the robot, whereas joint positions are enforced and realistic physics are ignored. This can cause unwanted behavior, such as penetration through objects. Hence, we change the control inputs to motor torques for the joints. For the robot reacher task, we also adapt the version of the "Reacher" task from OpenAI \cite{openai_gym}. Instead of being provided with euclidean position goals, the agents needs to reach goals in the robot's joint angle configuration space. 

\subsection{Environments}
\subsubsection{Navigation Mazes}
All navigation mazes are modelled by immovable blocks of size $4\times 4 \times 4$. \cite{nachum2018data} uses blocks of $8\times 8 \times 8$.  The environment shapes are clearly depicted in Figure \ref{fig:navigation_envs}. For the randomly generated maze, we sample each block with probability being empty $p=0.7$. The start and goal positions are also sampled randomly at uniform with a minimum of 5 blocks distance apart. Mazes where start and goal positions are adjacent or where the goal is not reachable are discarded. For evaluation, we generated 500 of such environments and reused them (one per episode) for all experiments. We will provide the random environments along with the code.

\subsubsection{Manipulation Environments}
The manipulation environments differ from the navigation mazes in scale. Each wall is of size $0.05 \times 0.05 \times 0.03$. We use a layout of $9 \times 9$ blocks. The object position is the position used for the planning layer. When the object escapes the top-down view range, the episodes are terminated. The random layouts were generated using the same methodology as for the navigation mazes. 

\subsubsection{Robot Reacher Environments}
The robot reacher environment is an adapted version of the OpenAI gym \cite{openai_gym} implementation. We add an additional degree of freedom to extend it to 3D space. The joint angles are projected onto a map of size $12\times12\times12$, where the axes correspond to the joint angles of the robot links. The goals are randomly sampled points in the robot's configuration space.

% \newpage

\section{Implementation Details}
\label{appendix_impl_details}
Our PyTorch~\cite{paszke2017pyTorch} implementation will be available on the project website\footnote{HiDe: \small{\url{https://sites.google.com/view/hide-rl}}}.
\subsection{Baseline Experiments}
For HIRO, HIRO-LR and HAC we used the authors' original implementations\footnote{HIRO: \url{https://github.com/tensorflow/models/tree/master/research/efficient-hrl}}\footnote{HAC: \url{https://github.com/andrew-j-levy/Hierarchical-Actor-Critc-HAC-}}. To improve the performance of HAC, we modified their Hindsight Experience Replay~\cite{andrychowicz2017hindsight} implementation so that they use the \textsc{Future} strategy.  More importantly, we also added target networks to both the actor and critic to improve the performance.
For HIRO, we ran the hiro\_xy variant, which uses only position coordinates for subgoals instead of all joint positions to have a fair comparison with our method. For HIRO-LR, we provide top-down view images of size 5x5x3 as in the original implementation. We train both HIRO and HIRO-LR for 10 million steps as reported in \cite{nachum2018nearoptimal}.
For RRT+LL, we adapted the RRT python implementation\footnote{RRT: \url{https://github.com/AtsushiSakai/PythonRobotics}} from \cite{python_robotics} to our problem. We trained a goal-conditioned low-level control policy in an empty environment with DDPG. During testing, we provide the low-level control policies with subgoals from the RRT planner. 
We used OpenAI's baselines \cite{baselines} for the DDPG+HER implementation. When pretraining for domain transfer, we made the achieved goals relative before feeding them into the network. For a better overview of the features the algorithms use, see Table \ref{tab:comp_overview}.

% \definecolor{darkgreen}{rgb}{0.0, 0.5, 0.0}
\newcommand{\gtick}{{\color{black}{\checkmark}}}
\newcommand{\btick}{{\color{black}\checkmark}}
\newcommand{\gcross}{{\color{black}{x}}}
\newcommand{\bcross}{{\color{black}x}}

\begin{table}[H]
\centering
\begin{tabular}{@{}ccccccc@{}}
\toprule
\multicolumn{1}{c}{Features} &
  \multicolumn{1}{c}{HiDe} &
  \multicolumn{1}{c}{RRT+LL} &
  \multicolumn{1}{c}{HIRO-LR} &
  \multicolumn{1}{c}{HIRO} &
  \multicolumn{1}{c}{HAC} &
  \multicolumn{1}{c}{DDPG+HER} \\ \midrule
Images           & \btick & \btick &  \btick  & \gcross & \gcross & \gcross \\
Random start pos & \gcross & \gcross & \gcross & \gcross & \btick  & \btick  \\
Random end pos   & \gcross & \btick & \btick  & \btick  & \btick & \btick \\
Agent position   & \btick & \btick  & \gcross & \btick  & \btick  & \btick  \\
Shaped reward    & \gcross & \gcross & \btick  & \btick  & \gcross & \gcross \\
Agent transfer    & \gtick  & \gtick & \bcross & \bcross & \bcross & \bcross \\ \bottomrule
\end{tabular}
  \vspace{0.1cm}
  \caption{Overview of related work and our method with their respective features. Features marked with a tick are included in the algorithm whereas features marked with a cross are not. See glossary below for a detailed description of the features. \newline \newline
  \textbf{Glossary:\newline}
Images: If the state space has access to images.\newline
Random start pos: If the starting position is randomized during training.\newline
Random end pos: If the goal position is randomized during training.\newline
Agent position: If the state space has access to the agent's position.\newline
Shaped reward: If the algorithm learns using a shaped reward.\newline
Agent transfer: Whether transfer of layers between agents is possible without retraining.}
  \label{tab:comp_overview}
\end{table}

\subsection{Ablation Baselines}

We compare HiDe against several different versions to justify our design choices. In HiDe-A(bsolute), we use absolute positions for the goal and the agent's position. In HiDe-3x3, HiDe-5x5, HiDe-9x9, we compare our learned attention window against fixed window sizes for selecting subgoals. In HiDe-RRT, we use RRT planning \cite{rrt} for the top-layer, while the lower layer is trained as in HiDe. This is to show that our learned planner improves the overall performance. 

\subsection{Evaluation Details}
For evaluation in the maze navigation experiment of Section \ref{sec:maze_nav}, we trained 5 seeds each for 2.5M steps for the simple maze navigation and 10M steps for the complex maze navigation “Training” environments. We performed continuous evaluation (every 100 episodes for 100 episodes). After training, we selected the best checkpoint based on the continuous evaluation of each seed. Then, we tested the learned policies for 500 episodes and reported the average success rate. Although the agent and goal positions are fixed, the initial joint positions and velocities are sampled from uniform distribution as is standard in OpenAI Gym environments \cite{openai_gym}. Therefore, the tables in the results (cf. Table \ref{tab:exp1}) contain means and standard deviations across 5 seeds.

\subsection{Network Structure}
\subsubsection{Planning Layer}
Input images for the planning layer were binarized in the following way: each pixel corresponds to one block (0 if it was a wall or 1 if it was a corridor).
In our planning layer, we process the input image via two convolutional layers with $3 \times 3 \times 3$ for the 3D case and $3 \times 3$ kernels for the 2D case. Both layers have only $1$ input and output channel and are padded so that the output size is the same as the input size. We propagate the value through the value map as in~\cite{nardelli2018value} $K=35$ times using a $3\times3\times3$ max pooling layer ($3\times3$ for 2D). Finally, the value map and position image is processed by 3 convolutions with $32$ output channels and $3\times3\times3$ filter window ($3\times3$ in 2D) interleaved by $2\times2\times2$ max pool ($2\times2$ for 2D) with $\relu$ activation functions and zero padding. The final result is flattened and processed by two fully connected layers with $64$ neurons, each producing outputs: $\sigma_1, \sigma_2, \sigma_3$ and the respective pairwise correlation coefficients $\rho$. We use $\Softplus$ activation functions for the $\sigma$ values and $\tanh$ activation functions for the correlation coefficients. The final covariance matrix $\Sigma$ is given by
$$\Sigma = 
\begin{pmatrix}
    \sigma_1^2 & \rho_{1,2}\,\sigma_1 \sigma_2 & \rho_{1,3}\,\sigma_1 \sigma_3 \\
    \rho_{1,2}\,\sigma_1 \sigma_2 & \sigma_2^2 & \rho_{2,3}\,\sigma_2 \sigma_3 \\
    \rho_{1,3}\,\sigma_1 \sigma_3 & \rho_{2,3}\,\sigma_2 \sigma_3  & \sigma_3^2 \\
    
\end{pmatrix}
$$ so that the matrix is always symmetric and positive definite. For numerical reasons, we multiply by the binarized kernel mask instead of the actual Gaussian densities. We set the values greater than the mean to $1$ and the others to zeros. 

% In practice, we use this line: 
% \begin{verbatim}
% kernel = t.where(kernel >= 
%  kernel.mean(dim=[1,2], keepdim=True), 
%  t.ones_like(kernel), t.zeros_like(kernel))    
% \end{verbatim}

\subsubsection{Control Layer}

We use the same network architecture for the lower layer as proposed by~\cite{levy2018hierarchical}, i.e. we use 3 times a fully connected layer with $\relu$ activation function. The control layer is activated with $\tanh$, which is then scaled to the action range.

\subsubsection{Training Parameters}
\begin{itemize}
    \itemsep0em
    \item Discount $\gamma = 0.98$ for all agents.
    \item Adam optimizer. Learning rate $0.001$ for all actors and critics.
    \item Soft updates using moving average; $\tau=0.05$ for all controllers.
    \item Replay buffer size was designed to store 500 episodes, similarly as in~\cite{levy2018hierarchical}
    \item We performed $40$ updates after each epoch on each layer, after the replay buffer contained at least 256 transitions.
    \item Batch size 1024.
    \item No gradient clipping
    \item Rewards 0 and -1 without any normalization.
    \item Observations also were not normalized.
    \item 2 HER transitions per transition using the \textsc{future} strategy~\cite{andrychowicz2017hindsight}.
    \item Exploration noise: 0.05 and 0.1 for the planning and control layer respectively.
\end{itemize}

\subsection{Computational Infrastructure}
All HiDe, HAC and HIRO experiments were trained on 1 GPU (GTX 1080). OpenAI DDPG+HER baselines were trained on 19 CPUs using the baseline repository \cite{baselines}.

%\subsubsection{Comparison Overview}
%\newpage
\section{Additional Results}
\label{additional_results}
% In this section, we present all results collected for this paper including individual runs.

\subsection{Maze Navigation}

\vspace{-0.5cm}
\begin{figure}[h]%
    \centering
    \hspace{-0.5cm}
    \subfloat[Simple Maze Navigation]{{
    \includegraphics[width=0.5\columnwidth]{figures/exp1_environments.png} }}%
    \qquad
    \hspace{-0.3 cm}
    \subfloat[Complex Maze Navigation]{
    {\includegraphics[width=0.4\columnwidth]{figures/exp2_envs_subset.png} }}%
    \caption{Maze environments for the tasks reported in a)  Section \ref{sec5_exp1} and \ref{sec:ablation_study}, b) Section \ref{subsec_mazenav_complex}. The red sphere indicates the goal, the pink cubes represent the subgoals. Agents are trained in only \textit{Training} and tested in \textit{Backward}, \textit{Flipped}, and \textit{Random} environments.}%
    \label{fig:navigation_envs}%
    \vspace{-0.3cm}
\end{figure}

\begin{table}[H]
\vspace{-0.5cm}
    \caption{Success rates of the individual seeds for achieving a goal in the maze navigation tasks.}
    \centering
    % \begin{tabular}{@{}cccc|cccc@{}}
    % \end{tabular}
    \begin{tabular}{@{}c|ccc|cccc@{}}
    %\multirow{2}{*}{Method} &
    % && Simple Maze &&&&  Complex Maze \\ \midrule 
    %\toprule \multicolumn{1}{N|}{} & \multicolumn{4}{G|}
    \toprule
    \multicolumn{1}{}{} & \multicolumn{3}{c}{Simple Maze} & \multicolumn{4}{c}{Complex Maze} \\ \midrule
    Method & Training     & Backward    & Flipped  & Training & Backward    & Flipped & Random    \\ \midrule
    HAC 1          & 96.4  & 00.0      & 00.0   & 00.0      & 00.0 & 00.0      & 00.0  \\
    HAC 2          & 82.0  & 00.0      & 00.0   & 00.0      & 00.0 & 00.0      & 00.0  \\
    HAC 3          & 85.6  & 00.4      & 00.0   & 00.0      & 00.0 & 00.0      & 00.0  \\
    HAC 4          & 92.8  & 00.0      & 00.0   & 00.0      & 00.0 & 00.0      & 00.0  \\
    HAC 5          & 55.6  & 00.0      & 00.0   & 00.0      & 00.0 & 00.0      & 00.0  \\ \midrule
    HIRO 1         & 89.0   & 00.0      & 00.0   & 68.0    & 00.0 & 00.0      & 44.6  \\
    HIRO 2         & 89.2  & 00.0      & 00.0   & 64.0     & 00.0 & 00.0      & 36.2  \\
    HIRO 3         & 94.0  & 00.0      & 00.0   & 80.0      & 00.0 & 00.0      & 33.6  \\
    HIRO 4         & 91.3  & 00.0      & 00.0   & 61.0      & 00.0 & 00.0      & 32.8  \\
    HIRO 5         & 90.8 & 00.0      & 00.0    & 81.0     & 00.0 & 00.0      & 34.4 \\ \midrule
    RRT+LL 1       & 13.8  & 24.0      & 19.6 & 4.8 & 5.6 & 1.2 & 43.6  \\
    RRT+LL 2       & 40.2  & 6.2       & 45.2 & 6.8 & 4.6 & 13.6 & 50.6  \\
    RRT+LL 3       & 20.2  & 23.8      & 29.0 & 17.0 & 8.4 & 0.4 & 47.0  \\
    RRT+LL 4       & 37.2  & 18.6      & 30.0 & 25.6 & 2.2 & 3.4 & 47.2   \\
    RRT+LL 5       & 15.0  & 38.2      & 23.4 & 9.4 & 13.2 & 5.8 & 50.6 \\ \midrule
    HIRO-LR 1      &  84.2  & 00.0      & 00.0 & 00.0      & 00.0 & 00.0      & 14.4   \\
    HIRO-LR 2      & 80  & 00.0      & 00.0  & 00.0      & 00.0 & 00.0      & 10.4  \\
    HIRO-LR 3      &  79.8 & 00.0      & 00.0  & 48.2      & 00.0 & 00.0      & 16.2  \\
    HIRO-LR 4      &  76 & 00.0      & 00.0  & 20.4      & 00.0 & 00.0      & 26.6  \\
    HIRO-LR 5      & 96.8  & 00.0      & 00.0  & 33.8      & 00.0 & 00.0      & 9.6  \\ \midrule
    HiDe 1         & 93.4  & 90.2      & 94.0  & 86.4 & 82.6 & 87.4 & 88.6  \\
    HiDe 2         & 90.8  & 68.2      & 91.8  & 83.4 & 66.0 & 66.0 & 81.6  \\
    HiDe 3         & 94.8  & 91.4      & 96.2 & 87.6 & 84.6 & 91.0 & 85.4 \\
    HiDe 4         & 94.0    & 85.2    & 92.6 & 87.2 & 76.6 & 77.6 &  83.2 \\
    HiDe 5         & 96.2  & 87.8      & 92.2 & 89.0 & 87.4 & 77.4 &  87.6 \\ \bottomrule
    \end{tabular}
    \label{tab:exp2_appendix}
\end{table}

\begin{table}[H]
\centering
\caption{Results of the simple maze navigation for HAC and HIRO when provided with an image. Both methods fail to solve the task, as the state space complexity is too high.}
\begin{tabular}{@{}c|ccc@{}}
\toprule
      & Training & Backward & Flipped \\ \midrule
HAC with Image & $0.0 \pm 0.0$  & $0.0 \pm 0.0$ & $0.0 \pm{0.0}$    \\
HIRO with Image & $0.0 \pm 0.0$  & $0.0 \pm 0.0$ & $0.0 \pm{0.0}$    \\ \bottomrule
\end{tabular}
\vspace{0.1cm}
\label{tab:hrl_image_fail}
\end{table}
    
% \subsection{Simple Maze Navigation}

%teaser_figure_new_2
\begin{figure}[H]%
    \centering
    \hspace{-0.5cm}
    \vspace{-0.1cm}
    \subfloat[]{{
    \includegraphics[width=0.45\columnwidth]{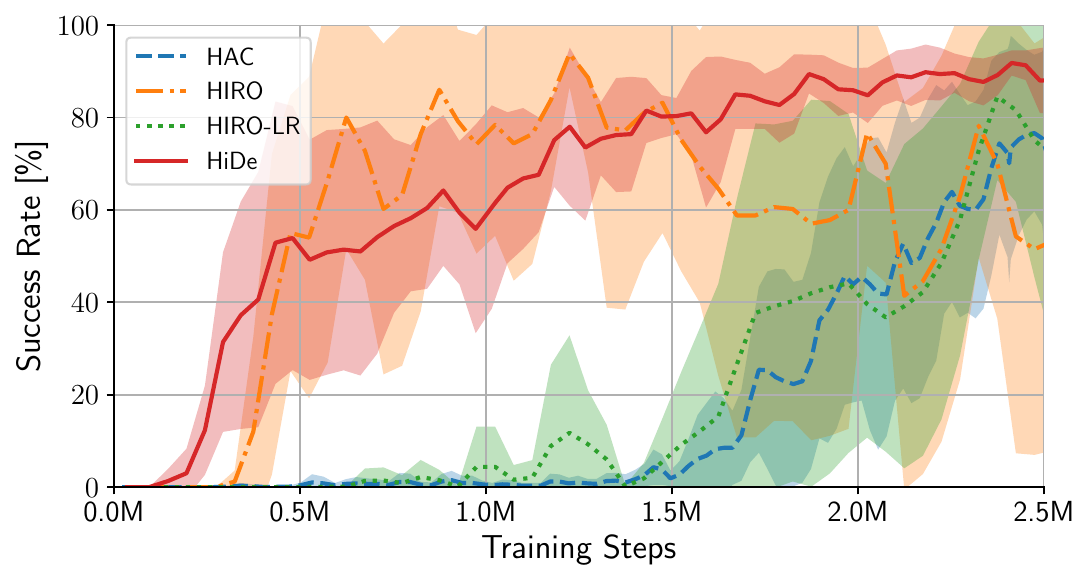} }}
    \qquad
    \hspace{-0.7 cm}
    \subfloat[]{
    {\includegraphics[width=0.45\columnwidth]{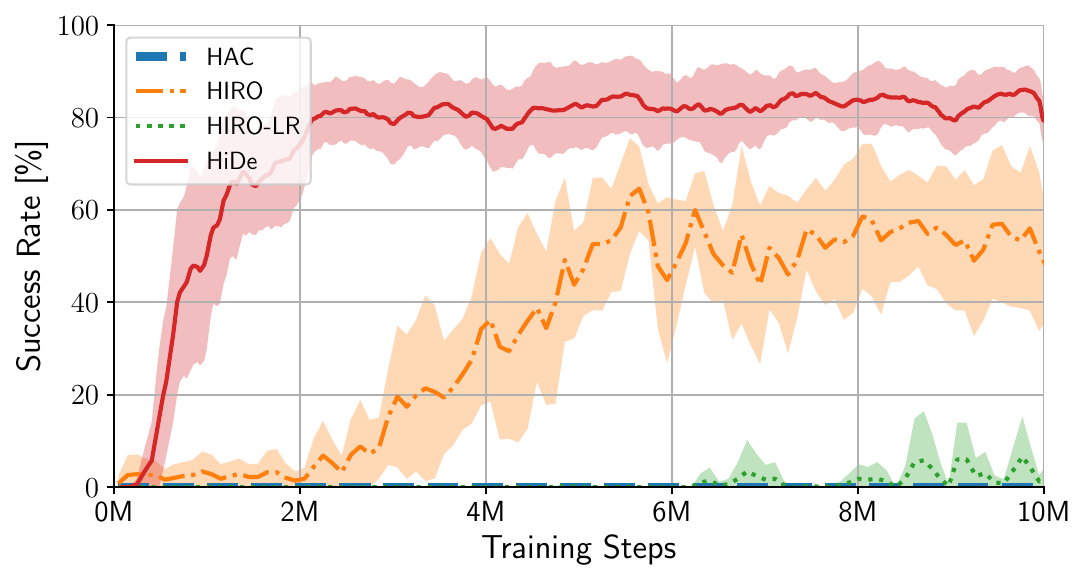} }}%
    \caption{Learning curves with success rates for the training tasks averaged over 5 seeds for a) the simple maze experiment from Section \ref{sec5_exp1}, b) the complex maze experiment from Section \ref{subsec_mazenav_complex}. HiDe matches convergence properties of HIRO in the simple maze (left), albeit having a much larger state space in the planning layer. In the more complex maze (right), HiDe shows similar convergence, while the convergence of HIRO slows.}%
    \label{fig:curves}%
    \vspace{-0.5cm}
\end{figure}

\begin{figure}[H]
\centering
  \includegraphics[width=0.7\columnwidth]{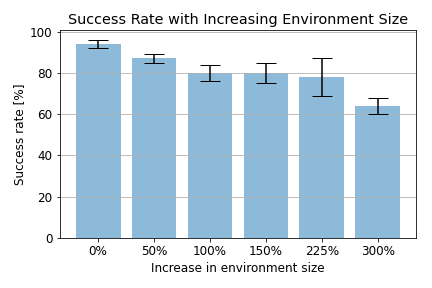}
  \vspace{-0.2cm}
  \caption{Success rates for the training task when gradually increasing the environment size and number of obstacles. At a 300\% increase, HiDe's performance drops to 64\%. See Table \ref{tab:hiro_lr_image_res} for the more detailed results.}%
  \label{fig:env_increase}
\end{figure}

\begin{table}[H]
\centering
\caption{Results for individual seeds of the HiDe experiments with gradually increasing number of obstacles and environment size.}
\begin{tabular}{@{}c|ccccc|c@{}}
\toprule
Maze Training & Seed 1 & Seed 2 & Seed 3 & Seed 4 & Seed 5 & Averaged \\ \midrule
HiDe env + 100\% & 84.0 & 83.4 & 82.5 & 75.8 & 75.8 & $80.3 \pm{4}$ \\
HiDe env + 150\% & 74.2 & 85.4 & 81.4 & 75.6 & 84.8 & $80.3 \pm{5}$ \\
HiDe env + 225\% & 78.0 & 69.6 & 70.8 & 82.2 & 91.4 & $78.4 \pm{9}$ \\
HiDe env + 300\% & 62.8 & 58.8 & 69.8 & 66.4 & 64.0 & $64.4 \pm{4}$ \\ \bottomrule
\end{tabular}
\vspace{0.1cm}
\label{tab:hiro_lr_image_res}
\end{table}

% \vspace{0.5cm}
% \begin{table}[H]
% \centering
%  \begin{tabular}{@{}c|@{\hspace*{\lengtha}}c@{\hspace*{\lengtha}}c@{\hspace*{\lengtha}}c@{}}
% \toprule
% Ant agent  & Training         & Backward          & Flipped          \\ \midrule
% HiDe-A     & $ 0 \pm  0$ & $ 0 \pm  0$   & $ 0 \pm  0$   \\
% HiDe-AR    & $95 \pm  1$ & $52 \pm 33$   & $34 \pm 45$   \\ \bottomrule
% \end{tabular}
%   \caption{Success rates in the simple maze (cf. Section \ref{sec5_exp1}). HiDe-A is our method with absolute subgoals. HiDe-AR has absolute goals and samples random goals during training. HiDe-A cannot solve the task, whereas HiDe-AR can learn the task, but does not generalize as well as our method.}%
%   \label{tab:exp1_abl}
% \end{table}

\subsection{Ablation Studies}

\begin{table}[H]
\centering
\begin{tabular}{@{}c|ccc@{}}
\toprule
Experiment     & Training & Backward & Flipped \\ \midrule
HiDe-A 1          & 88.2  & 5.4       & 49.4    \\
HiDe-A 2          & 89.2  & 28.4      & 53.2    \\
HiDe-A 3          & 84.8  & 35.8      & 29.6    \\
HiDe-A 4          & 91.2  & 13.6      & 32.2    \\
HiDe-A 5          & 88.2  & 00.0      & 14.4    \\ \midrule
HiDe-RRT 1         & 82.0  & 35.2     & 78.8    \\
HiDe-RRT 2         & 80.0  & 72.4     & 75.0    \\
HiDe-RRT 3         & 73.6  & 53.6     & 69.4    \\
HiDe-RRT 4         & 63.4  & 50.6     & 63.4    \\
HiDe-RRT 5         & 85.6  & 54.0     & 74.2    \\ \midrule
HiDe 3x3 1       & 28.4  & 0.0       & 4.4    \\
HiDe 3x3 2       & 67.6  & 0.6       & 44.0    \\
HiDe 3x3 3       & 59.6  & 0.4       & 36.4    \\
HiDe 3x3 4       & 0.0  &  0.0       & 0.0    \\
HiDe 3x3 5       & 76.8  & 6.6       & 67.8    \\ \midrule
HiDe 5x5 1      & 91.0  & 82.8      & 97.0    \\
HiDe 5x5 2      & 94.6  & 10.6      & 89.6    \\
HiDe 5x5 3      & 88.0  & 72.4      & 87.2    \\
HiDe 5x5 4      & 91.2  & 14.4      & 83.6    \\
HiDe 5x5 5      & 97.6  & 83.6      & 50.6    \\ \midrule
HiDe 9x9 1         & 90.6  & 9.4     & 81.2    \\
HiDe 9x9 2         & 92.4  & 64.4    & 79.4    \\
HiDe 9x9 3         & 89.8  & 1.2     & 85.6    \\
HiDe 9x9 4         & 99.0  & 4       & 83.0    \\
HiDe 9x9 5         & 94.6  & 3       & 68.2    \\ \bottomrule
\end{tabular}
\vspace{0.1cm}
\caption{Individual seed results of the ablation study for the simple maze navigation task.}
\end{table}

\begin{table}[H]
\centering
\begin{tabular}{@{}c|ccccc|ccccc@{}}
\toprule
           & Ant 1 & Ant 2 & Ant 3 & Ant 4 & Ant 5 & Averaged \\ \midrule
Training    &  0.0  & 78.8 &  0.0  & 0.0  &  0.0   & $16 \pm 35$\\
Random     & 67.2  & 88.8 & 17.6  & 0.0  & 0.0   & $35 \pm 41$\\
Backward   &  0.0  & 62.2  &  0.0  &  0.0  &  0.0   & $12 \pm 28$ \\
Flipped    &  0.0  & 79.8  &  0.0  &  0.0  &  0.0   & $16 \pm 36$ \\ \bottomrule
\end{tabular}
\vspace{0.1cm}
\caption{Results for the complex maze navigation task with HiDe-Absolute.}
\label{tab:abs_complex}
\end{table}

\vspace{0.5cm}
\begin{figure}[H]
\centering
\includegraphics[width=0.5\columnwidth, trim={0 245 390 0}]{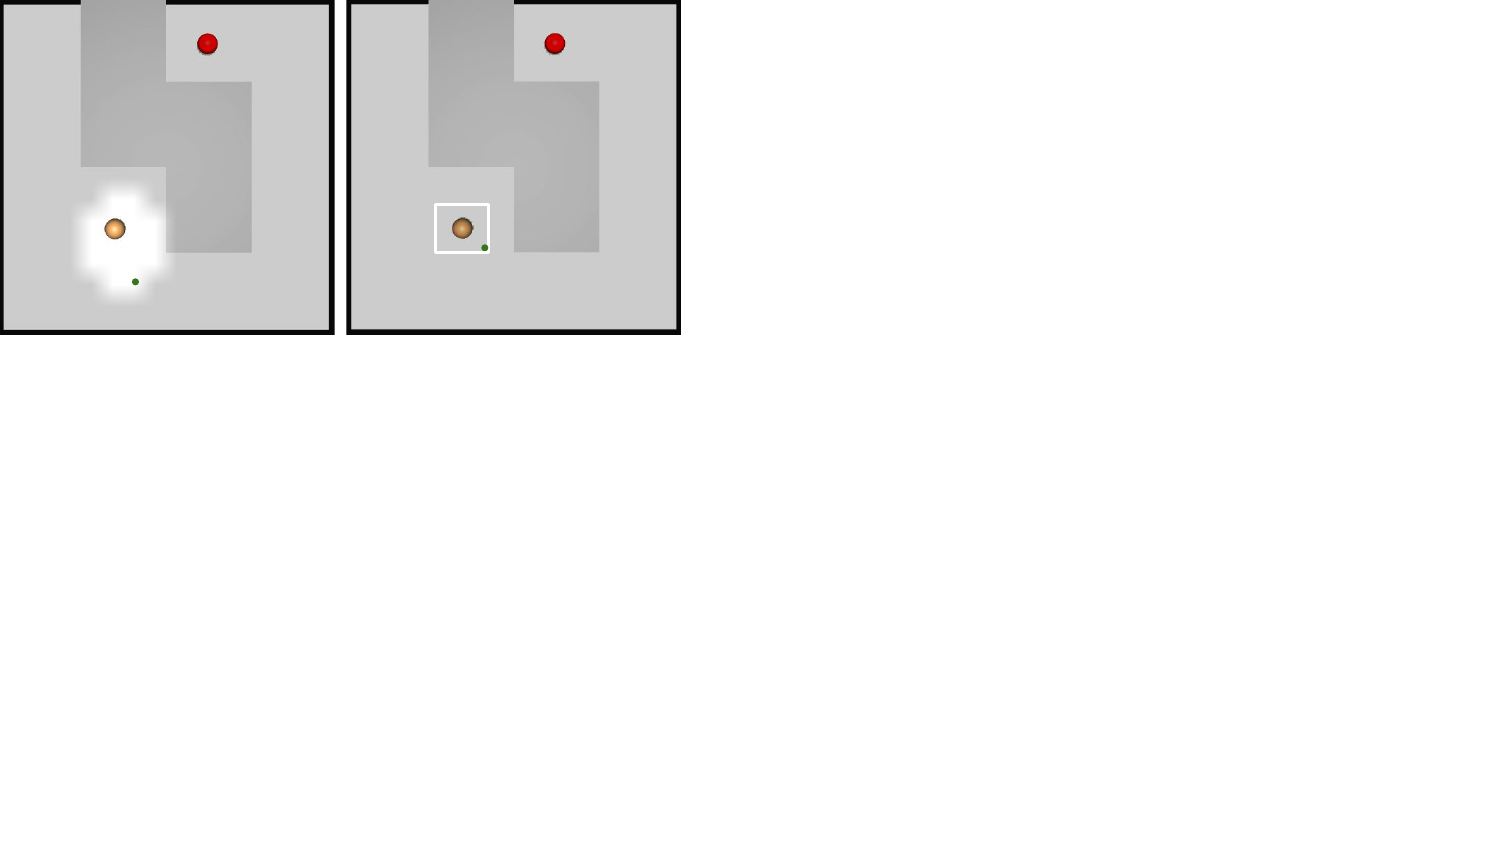}
\caption{A visual comparison of \textit{(left)} our dynamic attention window with a \textit{(right)} fixed neighborhood. The green dot corresponds to the selected subgoal in this case. Notice how our window is shaped so that it avoids the wall and induces a further subgoal.}\label{fig:window_comparison}
\end{figure}

\subsection{Agent Transfer}
\label{appendix:transfer}
\begin{table}[H]
\centering
\begin{tabular}{@{}c|ccccc|ccccc@{}}
\toprule
           & A$\rightarrow$B 1 & A$\rightarrow$B 2 & A$\rightarrow$B 3 & A$\rightarrow$B 4 & A$\rightarrow$B 5  & Averaged \\ \midrule
Training   & 99.8   & 100   & 100   & 100   & 100 & $100 \pm 0$ \\
Random    & 98.4    & 98.6  & 98.0  & 98.6  & 98.8 & $98 \pm 0$ \\
Backward & 100  & 100  & 99.8  & 100  & 100 & $100 \pm 0$  \\
Flipped   & 99.6   & 100   & 99.6   & 100   & 100 & $100 \pm 0$ \\ \bottomrule
\end{tabular}
\vspace{0.1cm}
\caption{Results of HiDe for ant to ball transfer for individual seeds.}
\end{table}

\begin{table}[H]
\centering
\begin{tabular}{@{}c|ccccc|ccccc@{}}
\toprule
           & B$\rightarrow$A 1 & B$\rightarrow$A 2 & B$\rightarrow$A 3 & B$\rightarrow$A 4 & B$\rightarrow$A 5 & Averaged   \\ \midrule
Training   & 73.4   & 73.4   & 71.2   & 68.2   & 71.6 & $72 \pm 2$ \\
Random    & 86.2   & 84.4   & 83.8   & 82.6   & 78.0 & $83 \pm 3$ \\
Backward  & 56.8   & 48.4   & 66.4   & 57.8   & 58.4 & $58 \pm 6$ \\
Flipped   & 74.4   & 77.4   & 80.0   & 61.6     & 72.8 & $73 \pm 7$ \\ \bottomrule
\end{tabular}
\vspace{0.1cm}
\caption{Results of HiDe for ball to ant transfer for individual seeds.}
\label{exp:agent_transfer}
\end{table}

\subsection{Robotic Arm Manipulation}
\begin{table}[H]
\centering
\begin{tabular}{@{}c|ccccc|ccccc@{}}
\toprule
           & Arm 1 & Arm 2 & Arm 3 & Arm 4 & Arm 5 & Averaged    \\ \midrule
Random    & 50  & 48  & 47  & 48  & 51  & $49 \pm 1$  \\
 \bottomrule
\end{tabular}
\vspace{0.1cm}
\caption{Results of the different seeds for the domain transfer experiments.}
\label{tab:domain_transfer}
\end{table}

\begin{figure}[H]
	\centering
	\includegraphics[width=1\columnwidth, trim={20 350 20 10},clip]{figures/arm.png}
	\caption{Example of three randomly configured test environments we use to demonstrate the domain transfer of the planning layer from a locomotion domain to a manipulation robot.}
	\label{fig:arm}
\end{figure}

% \begin{figure}[H]
% 	\centering
% 	\includegraphics[width=0.8\columnwidth]{figures/hide_reacher.png}
% 	\caption{Example of the robotic arm reach experiment. Instead of providing a top-down view to the planner, a projection map of the joint angles is used to plan a trajectory towards a given goal (yellow/green spheres). The subgoals for the joints are visualized as the respective yellow/green cubes.}
% 	\label{fig:hide_reacher}
% \end{figure}

\newpage

\section{Algorithm}
\label{algorithm}

\begin{algorithm}[H]
\caption{Hierarchical Decompositional Reinforcement Learning (HiDe)}\label{alg:HiDe}
\begin{algorithmic}

\State \textbf{Input:}
    \begin{itemize}
    \item Agent position $s_{pos}$, goal position $G$, and projection from environment coordinates to image coordinates and its inverse $Proj$,$Proj^{-1}$. 
    % \item Task design: $S_{init} \gets$ Initial state space, $G_{k-1} \gets$ task goal space 
    \end{itemize}
\State \textbf{Parameters:}
    \begin{enumerate}
        \item maximum subgoal horizon $H=40$, subgoal testing frequency $\lambda=0.3$ 
    \end{enumerate}
\State \textbf{Output:}
    \begin{itemize}
    \item $k=2$ trained actor and critic functions $\pi_0, ..., \pi_{k-1}, Q_0, ... , Q_{k-1}$
    \end{itemize}

% \State initialize $level[i].actor$, $level[i].critic$, $level[i].buffer$ for 0 $\leq$ $i$ $<$ $k$ 
\State
\For{$M$ episodes} \Comment{Train for M episodes}
% \Loop
    \State $s \leftarrow$ $S_{init}$, $g$ $\leftarrow$ $G_{k-1}$ \Comment{Get initial state and task goal}
    \State $train\_top\_level$($s$, $g$) \Comment{Begin training}
    \State Update all actor and critic networks
% \EndLoop
\EndFor

\State \Function{$\pi_1$}{$s::state, g::goal$}
    \State $v_{map}$ $\gets$ $MVProp(I, g_1)$ \Comment{Run MVProp on top-down view image and goal position}
    \State $\sigma, \rho$ $\gets$ $CNN(v_{map}, Proj(s_{pos}))$ \Comment{Predict mask parameters}
    \State $v$ $\gets$ $v_{map} \bigodot \mathcal{N}(\cdot | s_{pos}, \Sigma)$ \Comment{Mask the value map}
    \State \textbf{return} $a_1$ $\gets$ $Proj^{-1}(\argmax v) - s_{pos}$ \Comment{Output relative subgoal corresponding to the max value pixel}
\EndFunction

\State \Function{$\pi_0$}{$s::joints\_state, g::relative\_subgoal$}
    \State \textbf{return} $a_0$ $\gets$ $MLP(s, g)$ \Comment{Output actions for actuators}
\EndFunction

\State
\Function{train\_level}{$i::level, s::state, g::goal$}
% \State \textbf{Method} \textit{train} ($s, g$)
\State $s_i \gets s$, $g_i \gets g$ \Comment{Set current state and goal for level $i$}
\For{$H$ attempts or until $g_n$, $i \leq n < k$ achieved}
    \State $a_i$ $\gets$ $\pi_i(s_i, g_i)$ + $noise$ (if not subgoal testing) \Comment{Sample (noisy) action from policy}
    \If{$i > 0$} 
        \State Determine whether to test subgoal $a_i$
        \State $s_{i}^{'} \gets$ $train\_level$($i-1, s_i, a_i$) \Comment{Train level $i-1$ using subgoal $a_i$}
    \Else
        \State Execute primitive action $a_0$ and observe next state $s_{0}^{'}$
    \EndIf
    \State  \Comment{Create replay transitions}
    \If{$i > 0$ and $a_i$ not reached} 
        \If{$a_i$ was subgoal tested} \Comment{Penalize subgoal $a_i$}
            \State $Replay\_Buffer_i \gets [s = s_i, a = a_i, r = Penalty, s^{'} = s_{i}^{'}, g = g_{i}, \gamma = 0]$
        \EndIf
        \State $a_i \gets s_i^{'}$ \Comment{Replace original action with action executed in hindsight}
    \EndIf

    \State \Comment{Evaluate executed action on current goal and hindsight goals}
    \State $Replay\_Buffer_i \gets [s = s_i, a = a_i, r \in \{-1,0\}, s^{'} = s_{i}^{'}, g = g_{i}, \gamma \in \{\gamma, 0\}]$
    \State $HER\_Storage_i \gets [s = s_i, a = a_i, r = TBD, s^{'} = s_{i}^{'}, g = TBD, \gamma = TBD]$
    \State $s_i \gets s_i^{'}$
\EndFor
\State $Replay\_Buffer_i \gets$ Perform HER using $HER\_Storage_i$ transitions

\State \textbf{return} $s_i^{'}$\Comment{Output current state}
\EndFunction
% \State \textbf{End Method}

\end{algorithmic}
\end{algorithm}
